# Supplementary material for: Designing for Reproducibility: A Qualitative Study of Challenges and Opportunities in High Energy Physics
Source: arXiv:1903.05875 ancillary file (2019-03-14)
Supplement: Supplementary file 1 [file README.pdf]

## README

This document provides information about the supplementary materials of the paper *Designing for Reproducibility: A Qualitative Study of Challenges and Opportunities in High Energy Physics*. In order to foster the reproducibility of our work, we release various study resources. In the following, we provide information on the materials and illustrate why we did not add other resources that could have been of interest.

### We provide:

- *Interview questionnaire*. The questionnaire that was used for the 12 semi-structured interviews.
- *Paper exercise #1: Analysis connections and dependencies*. The paper exercise proofed to be very valuable in building an understanding of the connections and dependencies that exist between analyses. Based on their drawings, interviewees were able to describe how they could profit from a preservation service being aware of those relations.
- *Paper exercises #2: Faceting exercise*. This exercise was designed to generate an understanding of the underlying structure of analyses, as perceived by data analysts. It allowed us to better understand the value of information that a preservation service holds.
- *Analysis report: Atlas.ti report on code groups*. The interview transcriptions were organized and coded with the Atlas.ti data analysis software. Our extensive and highly collaborative analysis effort finally resulted in the generation of 22 code groups. We decided to publish the Atlas.ti report that entails those code groups, a short description of them and the corresponding codes.

### We do *not* provide:

- *Initial study design*. Before we conducted the study, we drafted a study design document that we used to communicate and to discuss the concept of the study internally. We initially wanted to provide this document as well. However, after having removed all references to contributing scientists, we feared that the template used might still provide inferences to an institute or organization. In addition, we realized that the

document did not provide substantial information that cannot be found in the paper or the other supplementary material.

- *The transcriptions of the interviews and the completed paper exercises.* We decided not to provide those resources, as they contain sensitive references that should not be publicly available and that were not quoted. We also believe that access could enable knowledgeable people to identify some of our participants. This would represent a violation of our agreement (Consent form), in which we assure that participants remain anonymous.

- *Consent form.* We used a consent form common to interview studies. As its structure and references provide inferences to the authors and/or their affiliations, we decided not to include it in the supplementary information.
