# Supplementary material for: Designing for Reproducibility: A Qualitative Study of Challenges and Opportunities in High Energy Physics
Source: arXiv:1903.05875 ancillary file (2019-03-14)
Supplement: Supplementary file 2 [file Atlas.ti_report.pdf]

# ATLAS.ti Report

---

## (Don't) re-invent the wheel

### Elements:

- Access to analyses as a starting point
- Access to reviewed fragments is reassuring
- Adapting code for one's purposes
- Aims at making analyses reproducible
- Creating and sharing libraries
- Data is available, but the documentation is not sufficient to find it
- Don't start from scratch - it takes too much effort
- Enabling to rerun analysis is motivating
- Find datasets instead of requesting new ones
- From scratch might be easier sometimes
- Good documentation might become personally useful in the long run
- Inheriting code from the group
- Need for better access to own analyses
- Re-use is essential in analysis work
- Wish to find things that already exist

### Comments:

This group highlights the importance of re-using already existing analyses or analysis fragments. Analysts wish to save time and rely on previously reviewed and tested code and configuration files. Furthermore, it provides insights into current practices and hurdles. The group stresses that sometimes it is easier to start from scratch, since there is a lack of documentation and good practices.

---

## Analysis design and planning demands access to information

### Elements:

- Access enables testing of ideas / improvement
- Check previous work and overlap
- Difficult to understand if others have already had same idea
- Documentation might not be enough to find previous work - might still have to ask
- Don't start from scratch - it takes too much effort
- Existing fragments as a starting point
- From the idea to a project
- Theorist's paper presents base for analysis
- Want to know a-priori what to expect

### Comments:

Planning new analyses requires a lot of information. Those include background on concepts in physics as well as previous work. It might also be helpful to draw back on information from theorists. The same applies for generally checking an idea for a future project.

---

## Automate running and interpretation

### Elements:

- Centralized computing to speed up work
- Desire: automatic interpretation
- Different analyses have many steps in common
- Hopes for the service to rerun analysis
- Not worrying about who provides computing resources
- Re-running centrally after code update makes things easier
- Wish to rely on centralized system to reproduce analyses

### Comments:

Analysts could profit from providing their code, if the system automatically performed some actions that otherwise they should have done manually. In particular, the system could automatically execute an analysis after documenting changes. That way, analysts would not have to search for computing resources by themselves. They could also save time on the setup and configuration of analysis execution workflows.

---

## Career benefits

### Elements:

- Ability to easily share results can lead to citation benefits
- Chance to outsource reproduction in the future
- Collaboration awareness to foster career
- No sharing means no reproduction and no citation
- Someone will receive credit if I can adapt their analysis for my cause

### Comments:

This groups highlights various ways in which access to a preservation system can drive careers. It mostly focuses on citation benefits that result from colleagues gaining access to documented analyses.

---

## Challenges of current information flow

### Elements:

- Code is the fastest communication channel
- Hesitation to engage in personal contact
- Meetings are a vital communication channel
- Need to ask
- Not sharing for competitive reasons
- Other people's code comes by email
- Reasons for secrecy
- Status and progress is communicated in meetings

### Comments:

Illustrates the need and importance of engaging with colleagues. The group shows how this engagement can be challenging. An important part of the interactions take place in meetings. They have a special role in HEP's collaborative work. They present one of the key information channels, not only for the state of individual analyses, but for physics knowledge in general. Presentations and notes from meetings are regarded as general documentation of information. However, they are difficult to search.

Accessing information and files often requires asking someone about it. Ideally, they will respond by sending the required resources or point to them. However, the outcome of asking for resources is often uncertain.

---

## Chance to foster collaborative work

### Elements:

- Analyses have input files in common
- Analyses have many elements in common
- Analysis is collaborative effort
- Chance of more people seeing code if accessible
- Collaborate on data selection (nTuples)
- Collaboration is based on personal level and institutes
- Competition vs Collaboration depends on individuals and groups
- Exchange can lead to improvements
- Multiple technologies for collaboration
- Reproduce based on suggestions to change
- Request resources together (with people doing similar things)
- Same analysis with two different codes
- Social media to update and discuss analyses
- Technology supports interaction / collaboration
- Value of discussion
- Visibility of analysis state can encourage collaboration

### Comments:

This group contains all information that highlight the opportunity of using a preservation service to foster collaborative work. It shows how the increased awareness on similar analyses and existing dependencies can lead to combined efforts. Documenting ongoing work and interests increases the likeliness to be perceived by analysts outside of one's own working group or institute. Combined efforts can significantly speed up analysis work and can lead to a more successful outcome of requests regarding the acquisition of (simulation) input data.

---

## Competition between collaborations (and individuals)

**Elements:**

- (Almost) impossible to find information on ongoing analyses from other collaborations
- Competition vs Collaboration depends on individuals and groups
- Everyone wants to have the main analysis
- HEP is characterized by many people and many data
- Know analysis state to avoid conflicts
- Not sharing for competitive reasons
- Variety of groups and institutes fosters competition

**Comments:**

Competitive behaviors and information exchange between LHC collaborations are depicted in this group. In general, there is almost no data and knowledge sharing between collaborations. That is especially true for collaborations that have similar goals. Independent verification is one of the political motives for this practice. To a lesser extent, also competition between analysts within the same collaboration are shown.

---

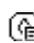 **Cultural change needed****Elements:**

- Difficult to change the mindset
- Documentation is not immediately useful
- Every day is tomorrow
- Have to avoid malpractice
- Lack of training on good practices
- Unwilling to make it reproducible AFTER the publication

**Comments:**

Data analysts perceive their domain in need for a cultural change. That includes especially training on good practices. Lacking reproducibility leads back to malpractice and the missing interest to document analyses.

---

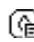 **Current search practices (Similarity)****Elements:**

- Chance to change search pattern: Desired event instead of whole analysis
- Google to find needed information
- Rather ask then search yourself
- Repository challenge: searchable only in master branch
- Searching for examples
- Searching for similar things is very common
- Searching is time consuming
- Searching mailing lists is challenging
- Searching with LaTeX syntax
- Using keywords to search

**Comments:**

Depicts current search practices and search approaches. The group highlights the similarity that exists between analyses. Researchers want to search for analyses that are similar to theirs. That way, they can look for examples or engage with other analysts.

---

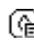 **Importance of dependency awareness****Elements:**

- Analyses have input files in common
- Being aware of similar analysis and overlap
- Dependency awareness to set alerts and receive notifications
- Important to keep track of different versions and changes
- Results depend on each other
- Update notification for dependent analyses

**Comments:**

Informs about existing dependencies between analyses that a preservation service could be aware of. Illustrates how analysts can use this awareness for their own benefit. In particular, they desire to be kept up-to-date on changes and vital information that affect their analyses. For example, input datasets are shared by various analyses. Detected errors should be communicated to all analysts who depend on them in their work.

---

## E-Mail (still) plays key role in communication

### Elements:

- E-mail to ask precise question - not an option for general questions
- Email communication to clear errors
- Other people's code comes by email
- Searching mailing lists is challenging
- Send e-mails to increase understanding
- Send mails to inform about discovered errors
- Shot in the dark: mailing lists
- Specific code files by e-mail are better than files without any context

### Comments:

Highlights the importance of email communication as one of the key information channels. Illustrates situations for which emails are suitable and some for which they are not. The group depicts that emails are not only key in communication with colleagues, but that they are also used to exchange resources. Instead of pointing to centrally stored repositories, needed resources are often attached to emails.

---

## Finding needed information is challenging

### Elements:

- Accessibility challenge: private access
- Can't search for a TWiki
- Current documentation (TWiki) is unstructured
- Difficult to find presentations
- Discoverability depends on state of analysis
- Few are unwilling to share code
- Hopeless to find code if I don't know the person
- Lack of documentation
- Need to ask for desired files
- Need to search to get to desired files
- Not completely aware who has access
- Personal relation is key to findability at the moment
- Repository challenge: ambiguity of user names
- Restricted access due to fear of judgement
- Searching is time consuming
- Various notation styles make it difficult to search for papers

### Comments:

Documents the various aspects connected to the time-consuming process of finding information. Illustrates that in some cases information cannot be found at all, even if they are existing. Challenges in the search architectures of the various repositories and knowledge databases represent a major reason for that. When analysts are not able to find needed resources, they usually try to ask colleagues.

---

## Human interaction and personal relations are vital

### Elements:

- (Committee) Validation requires author interaction
- Have to know which authors you can trust
- Knowledge is in people's head
- Need to ask
- People pointing to resources
- Personal relation is key to findability at the moment
- Physical accessibility to people is important
- Social media to update and discuss analyses
- Specific code files by e-mail are better than files without any context
- Talking to people is most useful
- TWikis provide information on contacts

### Comments:

Stresses the human factor in the search for information: knowledge is in people's heads! Details that the process of finding information often depends on the personal relations with colleagues. Even though information is usually stored somewhere in an accessible place, analysts often need to hope that their contacts are able to point them there. This is especially true for presentations that had been given several years back. The high rotation of analysts at CERN makes finding the right person even more demanding in that case.

---

## Importance of reproducibility and motives to reproduce analyses

### Elements:

- Aims at making analyses reproducible
- Analyses are reproduced with new data
- Comparing results for verification
- More data can uncover errors
- Reproduce based on suggestions to

change ○ Reproduce because of theory progress ○ Reproduce to react on discovered errors ○  
Reproduction based on code change ○ Reproduction can take a lot of time ○ Reproduction  
requires same people from before ○ Short life-time of technical setups is challenging

**Comments:**

Details the various reasons that can lead to the reproduction of analyses and fragments.  
Highlights the importance of reproducing analyses. Stresses that reproduction is (currently) often  
a very time consuming task, as analyses are not sufficiently documented and prepared for  
automated re-execution.

---

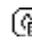 **Institute's heterogeneity poses challenges - but they still play a vital role**

**Elements:**

○ Advisors in two places: institute and CERN ○ Code at institute not runnable outside ○ Code is  
stored at institute ○ Collaboration is based on personal level and institutes ○ Easier to  
coordinate for computing time in institutes ○ Effort to centralize from institute ○ Institute's  
computing resources all work different ○ Institute's resources are preferred / faster ○ Moving  
institute requires adapting to new computing infrastructure ○ Space at CERN is limited

**Comments:**

Most analysts, even those working locally at CERN, are affiliated with an institute abroad.  
Institutes play a vital role in the analysis process and the storing of information. Analysts can  
profit from them. At the same time, the heterogeneity of the institute's computing resources  
represents issues, as sharing and collaboration is hindered.

---

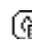 **Interaction with theorists**

**Elements:**

○ Challenging to keep up with work from theorists ○ Citation as motivation to share for theorists  
○ Communication with theorists is good ○ Need to check paper's claims and feasibility ○  
Reproduce because of theory progress ○ Papers from theorists represent base for analysis ○  
Theorists want to know who works on what

**Comments:**

Depicts the important connection between theorists and experimentalists. The group highlights  
the usually good relationship from which both sites can profit. Illustrates in particular, how the  
work of theorists represents a base of work for data analysts. In return, theorists can profit from  
experimentalists taking interest in their work by increasing their citation count. The  
communication strongly relies on personal relations.

---

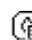 **Lack of documentation**

**Elements:**

○ Black box, not explaining ○ Code is badly commented ○ Corrected code files are not shared  
○ Data is available, but the documentation is not sufficient to find it ○ Difficult for newcomers ○  
Documentation is often outdated ○ Hope for documentation ○ Lack of documentation ○ Need to  
access code as documentation is usually bad ○ No documentation of how standard methods are  
done ○ No track record of what is happening ○ People complain missing / outdated  
documentation ○ Repository discussions and issues are not preservation efforts ○ Reverse-  
engineering to cope with lack of documentation ○ Similar things can lead to errors if they are not  
fitting well ○ Variations in level of documentation observed

**Comments:**

Analysts complain about the lack of documentation of analyses and code files. The group  
illustrates the consequences of missing documentation. In particular, outdated documentation is

typical and represents a serious problem, in that it might lead analysts in a wrong direction. Highlights the effort needed to keep documentation up-to-date.

---

## Opportunity to facilitate coordination and management

### Elements:

- Certainty about datasets used
- Certainty that my datasets are not deleted
- Lack of progress indicators (vs. industry)
- Supervisor might check student's code
- Uncertainty of project outcome (time)

### Comments:

Access to a preservation service provides a wide set of benefits for planning and management efforts in analysis work. The combined knowledge of used resources allows to better adapt the infrastructure to analyst's needs. In particular, knowing what input datasets are needed by analysts allows to ensure that those resources are kept on the servers.

---

## Publication alone is not enough

### Elements:

- Code connected to publications needed
- Lack of declaration of notation is key challenge in papers
- Link codes to sections of a paper
- Linking internal notes to publications
- Need to check paper's claims and feasibility
- Short papers don't contain enough information
- The truth is the software

### Comments:

HEP is characterized by very open scholarly communication. A lot of papers and pre-prints contain physics knowledge. However, the publications are mostly insufficient to really get an analysis going. Often, the code files that lead to a publication are needed. Having access also clears issues that result from using various different notations without explicitly describing them.

---

## Scalability challenge

### Elements:

- Analyses are reproduced with new data
- Analyses take longer - Contract durations stay the same
- Complexity and speed increases
- Continue work of people having left is a challenge
- Current practices to redo everything not feasible anymore in future
- Groups switch interest and leave analyses unfinished
- HEP is characterized by many people and many data
- More and more possibilities for data analysis and less people
- Orphan analyses
- Reproducibility to counter growing complexity
- Results are not published because no one is there to publish them anymore
- Review times increase
- Rotation of people is a problem
- Short life-time of technical setups is challenging
- Time pressure makes codes only worse
- More and more understaffed

### Comments:

This group draws back to the core of data intensive science. With the growing amount of data and computing capabilities, the analysis work gets continuously more demanding. Since contract durations stay the same, analysts feel increasing time pressure. In addition, rotation of people is a key issue in HEP. Especially since analyses often need to be reproduced many years after they were written. Illustrates that analysts need to be supported to become more proficient in reproducible practices and that this is needed to counter the growing scalability challenge.

---

## Structure analysis work and automate documentation

**Elements:**

- Analyses are well structured
- Different analyses have many steps in common
- Everybody does the same thing
- Fear that templating could limit analyst's choices
- Hope that service facilitates documentation
- Lego block style analysis work
- Templates can facilitate design
- Templates can help to structure analysis work

**Comments:**

Analyses follow a similar structure. Based on that similarity, a preservation service could perform automated checks and provide templates for the analysis design. That way, documenting ongoing analyses can facilitate the design and reliability. To some extent, it could also be able to document analyses automatically.

---

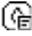 **The widespread knowledge base and its challenges****Elements:**

- E-mail to ask precise question - not an option for general questions
- Internal documentation is vital learning resource
- Lack of declaration of notation is key challenge in papers
- Learning / applying by example
- Linking everything together
- Need to look at code to learn
- Preprint as learning resource
- Presentations as learning resource
- Reading helps to understand, but not to implement
- Send e-mails to increase understanding
- Shared analyses for teaching
- Short papers don't contain enough information
- Similar analyses for learning
- To learn, code is first - books last
- Various notation styles make it difficult to search for papers
- Wikipedia as information source

**Comments:**

Shows how studying and learning is done today and what would be needed. A multitude of learning resources exist that demand different approaches. Linking various sources could harmonize the access to knowledge.
