# Supplementary material for: Designing for Reproducibility: A Qualitative Study of Challenges and Opportunities in High Energy Physics
Source: arXiv:1903.05875 ancillary file (2019-03-14)
Supplement: Supplementary file 3 [file Interview_questionnaire.pdf]

## Questionnaire

### About the researcher

1. Please briefly describe your role and main duties within your collaboration.

### Current practices

#### Preservation / Reuse

2. How are you storing your most recent analysis?
3. Tell me about an experience, reusing one of your colleagues analysis.

#### Information seeking

4. When you begin working on a new task - how do you start? What resources do you need?
5. Tell me about the last time that you had to search for information or resources during your analysis work.
6. Please describe an experience that required you to access data or code files from a colleague.

### Expectations

7. Please elaborate on the opportunities you see for having an analysis preservation platform in respect to
  - a. future re-use of data and artefacts?
  - b. completely re-running analyses in the future?
8. How might direct access to your collaboration's analyses support you in your day to day analysis work?

### CERN Analysis Preservation (CAP) prototype service: Walkthrough & related questions

*I would like you to have a look at CERN Analysis Preservation.*

#### Walkthrough

9. *Guiding the interviewee through CAP*
  - a. *This is the CAP dashboard. I will explain to you what those elements (Shared records, My drafts, My shared deposits) mean.*
  - b. *I will show you the analysis description form that corresponds to your collaboration (LHCb / CMS / ATLAS / ALICE).*
  - c. *Please familiarize yourself with the analysis description form.*

#### Using stored information - *Let's think of how you could use the data stored in CAP.*

10. What would you type into the search bar?

- a. What exactly is it that you want to find?
  - b. In what situation do you search for it?
  - c. Why is that important to you?
  - d. How would you currently search for those information?
  - e. *Exercise.* Please use the search bar to find what you want to find.
11. *Exercise #1 - Connections and dependencies*
- a. What kind of relations exist between analyses? *Please draw them on the paper.*
  - b. How could you profit from CAP being aware of these connections?
12. *Exercise #2 - Faceting exercise: The search result page allows you to filter and sort analyses that you are interested in. Design the facets in a way that would support you in searching a list of analyses.*

### **Reflection on CAP**

- 13. What don't you understand about CAP?
- 14. What functionality is CAP missing?
- 15. Please tell me if you would want to make an effort to describe your analyses on CAP.
  - a. *If he/she wants to contribute:* Why would you want to contribute?
  - b. *If he/she does not want to contribute:* Why are you hesitant to contribute?
- 16. Tell me about any concerns you have when it comes to a platform like CAP.
- 17. How could access to CAP support you in your daily analysis work?

### **Value of a preservation system**

- 18. Tell me about an experience, in which having had access to a system fully storing the analyses of you and your colleagues could have solved a problem.
- 19. *(For conveners / project managers):*
  - a. Please describe how you recently checked the status or progress of analyses in your group.
  - b. Which information are important when checking the status and progress of projects?
- 20. *(For interviewee's who are not project managers):*
  - a. Tell me about the last time you checked the status or progress of a colleagues' analysis.
  - b. *In case the interviewee recalls an event:*
    - What is the reason for keeping track of a colleagues analysis?
    - How do you currently do that?
    - What information of your colleagues' analyses is most interesting?

### **Debrief**

- 21. Do you have any other thoughts or comments on the topics we were discussing?
